# Supplementary material for: Regression-clustering for Improved Accuracy and Training Cost with Molecular-Orbital-Based Machine Learning
Source: arXiv:1909.02041 source file (2019-10-23)
Supplement: Supplementary file 1 [file SI.pdf]

# Supporting Information for Regression-clustering for Improved Accuracy and Training Cost with Molecular-Orbital-Based Machine Learning

Lixue Cheng,[†] Nikola B. Kovachki,[‡] Matthew Welborn,[†] and Thomas F. Miller III[*,†]

† *Division of Chemistry and Chemical Engineering, California Institute of Technology, Pasadena, CA 91125, USA*

‡*Computing and Mathematical Sciences, California Institute of Technology, Pasadena, CA 91125, USA*

E-mail: tfm@caltech.edu.

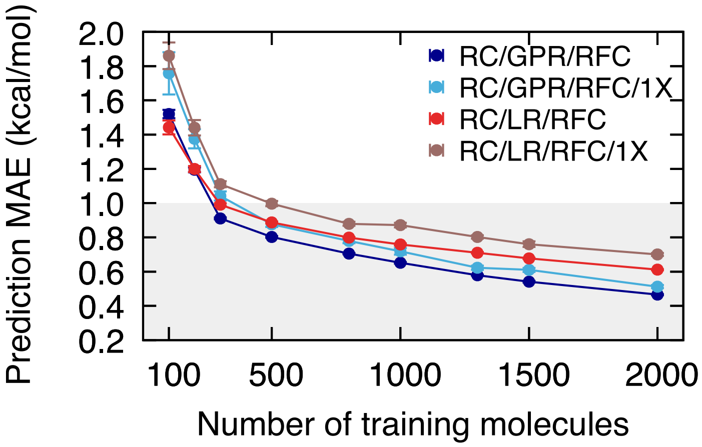


FIG. S1: Learning curves for various implementations of MOB-ML applied to MP2/cc-pVTZ correlation energies, with the training and testing sets corresponding to non-overlapping subsets of QM7b-T. Results obtained from averaging over 10 independent models are compared to results from a single model (/1X) without averaging. For both the RC/GPR/RFC and RC/LR/RFC implementations, averaging over independent models reduces the prediction MAE.

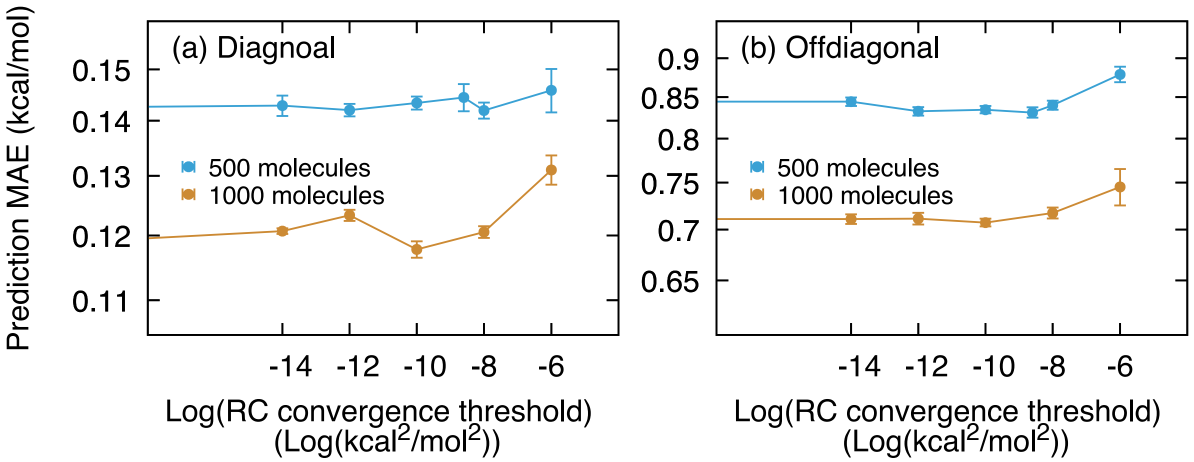


FIG. S2: Sensitivity of MOB-ML predictions to the RC convergence threshold. Results are obtained using the RC/LR/RFC implementation of MOB-ML applied to MP2/cc-pVTZ correlation energies, with the training and testing sets corresponding to non-overlapping subsets of QM7b-T. The prediction MAEs for the contributions from the (a) diagonal and (b) off-diagonal pair energies are shown for two different training set sizes. For both the diagonal and off-diagonal pair contributions, a threshold value of $1 \times 10^{-8}$ kcal$^2$/mol$^2$ for the RC loss function (Eq. 4 in the main text) provides similar results as tighter convergence thresholds.

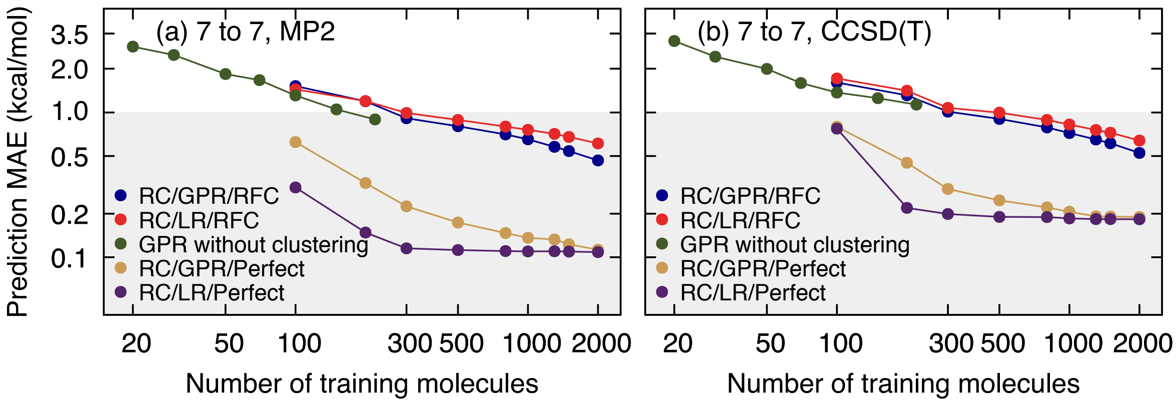


FIG. S3: Learning curves for various implementations of MOB-ML applied to (a) MP2/cc-pVTZ and (b) CCSD(T)/cc-pVDZ correlation energies, with the training and test sets corresponding to non-overlapping subsets of the QM7b-T set of drug-like molecules with up to heavy seven atoms. These results are identical to those of Fig. 7 in the main text, except plotted on a log-log scale.

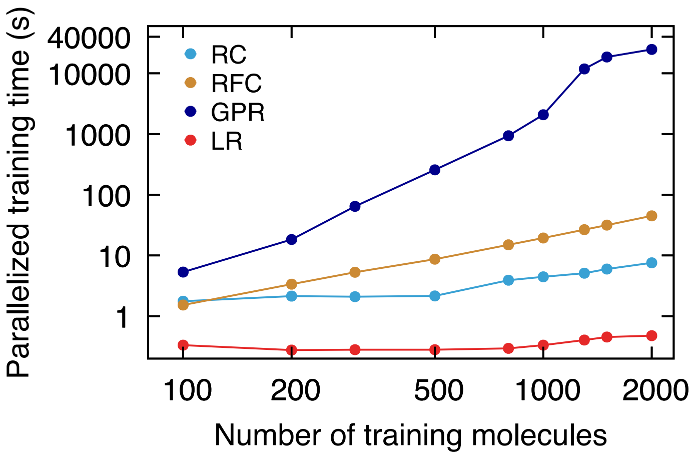


FIG. S4: Breakdown of the wall-clock timings for RC, RFC, GPR and LR for different number of training molecules from the QM7b-T set at the MP2/cc-pvTZ level of theory. The parallelization is implemented as follows. Within the RC step, the LR regression of each cluster is performed independently on a different core of a 16-core Intel Skylake (2.1 GHz) CPU processor. With in the regression step, the LR and GPR regression of each cluster is likewise performed independently on a different core. For RFC training, we apply employ parallel 200 cores using the parallel implementation of Scikit-learn, since there are 200 trees.

TABLE S1: MOB-ML prediction accuracy for the RC/GPR/RFC implementation, applied to correlation energies at the MP2/cc-pVTZ level. Training sets are comprised of subsets of the QM7b-T dataset, with the number of training molecules indicated. Correlation energy predictions are made for test sets comprised of the remaining seven-heavy-atom molecules from QM7b-T and the thirteen-heavy-atom molecules from GDB-13-T. Energies in kcal/mol.

| QM7b-T | QM7b-T prediction | | GDB-13-T prediction | | | |
|---|---|---|---|---|---|---|
| training molecules | MAE | SEM | MAE | SEM | MAE/heavy atom | SEM/heavy atom |
| 100 | 1.520 | 0.025 | 3.415 | 0.046 | 0.2431 | 0.0035 |
| 200 | 1.194 | 0.014 | 2.785 | 0.024 | 0.1992 | 0.0018 |
| 300 | 0.9109 | 0.0056 | 2.366 | 0.027 | 0.1724 | 0.0020 |
| 500 | 0.8028 | 0.0048 | 2.278 | 0.023 | 0.1655 | 0.0018 |
| 800 | 0.7048 | 0.0036 | 2.161 | 0.020 | 0.1564 | 0.0015 |
| 1000 | 0.6517 | 0.0043 | 2.088 | 0.021 | 0.1497 | 0.0016 |
| 1300 | 0.5791 | 0.0032 | 2.062 | 0.019 | 0.1482 | 0.0015 |
| 1500 | 0.5414 | 0.0052 | 1.993 | 0.012 | 0.1432 | 0.0009 |
| 2000 | 0.4654 | 0.0027 | 1.913 | 0.016 | 0.1332 | 0.0012 |

TABLE S2: MOB-ML prediction accuracy for the RC/LR/RFC implementation, applied to correlation energies at the MP2/cc-pVTZ level. Training sets are comprised of subsets of the QM7b-T dataset, with the number of training molecules indicated. Correlation energy predictions are made for test sets comprised of the remaining seven-heavy-atom molecules from QM7b-T and the thirteen-heavy-atom molecules from GDB-13-T. Energies in kcal/mol.

| QM7b-T | QM7b-T prediction | | GDB-13-T prediction | | | |
|---|---|---|---|---|---|---|
| training molecules | MAE | SEM | MAE | SEM | MAE/heavy atom | SEM/heavy atom |
| 100 | 1.442 | 0.041 | 3.427 | 0.086 | 0.2636 | 0.0066 |
| 200 | 1.199 | 0.018 | 2.935 | 0.035 | 0.2258 | 0.0027 |
| 300 | 0.9909 | 0.0084 | 2.596 | 0.029 | 0.1997 | 0.0023 |
| 500 | 0.8869 | 0.0051 | 2.412 | 0.016 | 0.1855 | 0.0013 |
| 800 | 0.7984 | 0.0042 | 2.394 | 0.020 | 0.1842 | 0.0015 |
| 1000 | 0.7586 | 0.0062 | 2.301 | 0.026 | 0.1770 | 0.0020 |
| 1300 | 0.7100 | 0.0038 | 2.321 | 0.021 | 0.1786 | 0.0017 |
| 1500 | 0.6769 | 0.0037 | 2.257 | 0.014 | 0.1736 | 0.0011 |
| 2000 | 0.6115 | 0.0028 | 2.218 | 0.022 | 0.1706 | 0.0017 |

TABLE S3: MOB-ML prediction accuracy for the RC/GPR/Perfect and RC/LR/Perfect implementations, applied to correlation energies at the MP2/cc-pVTZ level, with the training and testing sets corresponding to non-overlapping subsets of QM7b-T. Energies in kcal/mol.

| | RC/GPR/Perfect | | RC/LR/Perfect | |
|---|---|---|---|---|
| training molecules | MAE | SEM | MAE | SEM |
| 100 | 0.6235 | 0.0331 | 0.3031 | 0.0574 |
| 200 | 0.3254 | 0.0113 | 0.1481 | 0.0231 |
| 300 | 0.2246 | 0.0075 | 0.1153 | 0.0031 |
| 500 | 0.1734 | 0.0052 | 0.1120 | 0.0029 |
| 800 | 0.1470 | 0.0031 | 0.1104 | 0.0031 |
| 1000 | 0.1361 | 0.0026 | 0.1096 | 0.0032 |
| 1300 | 0.1324 | 0.0014 | 0.1099 | 0.0033 |
| 1500 | 0.1230 | 0.0019 | 0.1095 | 0.0034 |
| 2000 | 0.1127 | 0.0010 | 0.1085 | 0.0035 |

TABLE S4: MOB-ML prediction accuracy for the RC/GPR/RFC and RC/LR/RFC implementations, applied to correlation energies at the CCSD(T)/cc-pVDZ level, with the training and testing sets corresponding to non-overlapping subsets of QM7b-T. Energies in kcal/mol.

| | RC/GPR/RFC | | RC/LR/RFC | |
|---|---|---|---|---|
| training molecules | MAE | SEM | MAE | SEM |
| 100 | 1.607 | 0.041 | 1.718 | 0.065 |
| 200 | 1.314 | 0.016 | 1.412 | 0.025 |
| 300 | 1.013 | 0.006 | 1.075 | 0.012 |
| 500 | 0.9026 | 0.0036 | 0.9951 | 0.0063 |
| 800 | 0.7880 | 0.0031 | 0.8876 | 0.0051 |
| 1000 | 0.7194 | 0.0053 | 0.8253 | 0.0062 |
| 1300 | 0.6495 | 0.0047 | 0.7559 | 0.0035 |
| 1500 | 0.6116 | 0.0034 | 0.7251 | 0.0034 |
| 2000 | 0.5243 | 0.0026 | 0.6402 | 0.0028 |

TABLE S5: MOB-ML prediction accuracy for the RC/GPR/RFC implementation with cluster-size capping, applied to correlation energies at the MP2/cc-pVTZ level, with the training and testing sets corresponding to non-overlapping subsets of QM7b-T. Energies in kcal/mol.

| training molecules | $N_{\mathrm{cap}} = 100$ | $N_{\mathrm{cap}} = 200$ | $N_{\mathrm{cap}} = 300$ | $N_{\mathrm{cap}} = 500$ | $N_{\mathrm{cap}} = 800$ |
|---|---|---|---|---|---|
| 100 | 1.520 | 1.520 | 1.520 | 1.520 | 1.520 |
| 200 | 1.217 | 1.194 | 1.194 | 1.194 | 1.194 |
| 300 | 0.9827 | 0.9318 | 0.9109 | 0.9109 | 0.9109 |
| 500 | 0.9211 | 0.8370 | 0.8049 | 0.8028 | 0.8028 |
| 800 | 0.9066 | 0.8028 | 0.7368 | 0.7054 | 0.7048 |
| 1000 | 0.8532 | 0.7745 | 0.7178 | 0.6676 | 0.6534 |
| 1300 | 0.8602 | 0.7568 | 0.6983 | 0.6261 | 0.5980 |
| 1500 | 0.8432 | 0.7353 | 0.6740 | 0.5892 | 0.5511 |
| 2000 | 0.8549 | 0.7456 | 0.6620 | 0.5753 | 0.5148 |
